# Supplementary material for: Online Human Activity Recognition using Low-Power Wearable Devices
Source: arXiv:1808.08615 source file (2019-02-04)
Supplement: Supplementary file 1 [file appendix.tex]

%\appendix
\normalsize
\vspace{-2mm}
\section*{Appendix: Derivation of Equation} \label{proof_F_T}
Let us consider that there are $N_h$ neurons in the hidden layer and $N_a$ 
neurons in the output layer. We also have a bias term that is acting as an 
input to the output layer. As a result, there are $N_h + 1$ connections to each 
output neuron. Using this notation, the output of each neuron in the output 
layer before the softmax function is applied is given by:
\begin{equation}\label{eq:hidden_out}
O_j = \sum_{i=1}^{N_{h} + 1} h_{o,i} \theta_{2,j,i}
\end{equation}
where  $\theta_{2,j,i}$ is the $i$th weight to $j$th output and $h_{o,i}$ is 
the 
output of the hidden 
layer corresponding to $\theta_{2,j,i}$. Now the probability of any action $A$, 
that is the policy $\pi(A|x, \theta)$ is 
given by the softmax function as:
\begin{equation}
\pi(A|x, \theta) = \frac{\exp(O_A)}{\sum_{j=1}^{N_a}{\exp(O_j)}}
\end{equation}
where $O_a$ is given by equation~\ref{eq:hidden_out}. Now, we need to find the 
gradient of $\pi(A|x, \theta)$ with respect to the output layer weights 
$\theta_2$. Furthermore, we can divide $\theta_2$ into two sets $\mathcal{S}_1$ 
, $\mathcal{S}_2$ to separate the output layer weights into the ones directly 
connected to the neuron corresponding to action $A$ and those connected to 
other output layer neurons. Using this notation, the derivative of $\pi(a|x, 
\theta)$ with respect to the weights in $\mathcal{S}_1$ and $\mathcal{S}_2$ can 
be written as:
\begin{equation}\label{eq:derivative_main}
\frac{\partial\pi(A|x, \theta)}{\partial{\theta_{2,j,i}}} = \begin{cases}
\frac{\partial\pi(A|x, \theta)}{\partial{O_A}}\frac{\partial 
O_A}{\partial{\theta_{2,j,i}}} & \theta_{2,j,i} \in \mathcal{S}_1 \\
\frac{\partial\pi(A|x, \theta)}{\partial{O_j}}\frac{\partial 
	O_j}{\partial{\theta_{2,j,i}}} & \theta_{2,j,i} \in \mathcal{S}_2, a_j \neq 
	A 
	\\
\end{cases}.
\end{equation}
Next, we can write $\frac{\partial\pi(a|x, \theta)}{\partial{O_A}}$ as:
\begin{align}
\frac{\partial\pi(a|x, \theta)}{\partial{O_a}} &= 
\frac{\exp(O_A)}{\sum_{j=1}^{N_a}{\exp(O_j)}} - 
\frac{\exp(O_A)^2}{(\sum_{j=1}^{N_a}{\exp(O_j)})^2} \\
& = \pi(A|x, \theta)(1 - \pi(A|x, \theta))
\end{align}
Similarly, we can write $\frac{\partial\pi(A|x, \theta)}{\partial{O_j}}$ as:
\begin{equation}
\frac{\partial\pi(a|x, \theta)}{\partial{O_j}} = -\pi(A|x, \theta)\pi(a_i|x, 
\theta), a_i \neq A
\end{equation}
Finally, $\frac{\partial 
	O_j}{\partial{\theta_{2,j,i}}}$ is just given by the output of the hidden 
	layer corresponding to $\theta_{2,j,i}$, since that $O_j$ is a linear 
	combination of the weights and outputs of the hidden layer. Therefore, 
	$\frac{\partial 
		O_j}{\partial{\theta_{2,j,i}}}$ is given by $ h_{o,i}$.	
Using this in Equation~\ref{eq:derivative_main} we get the gradients as:
\begin{equation}\label{eq:rl_grad_final}
\frac{\partial \pi(A|x,\theta)}{\partial\theta_{2,j,i}} =
\begin{cases}
\pi(A|x,\theta) (1 - \pi(A|x,\theta)) h_{o,i}, & \theta_{2,j,i} \in
\mathcal{S}_1 \\
-\pi(A|x,\theta) \pi(a_j|x_t,\theta_t) h_{o,i}, &
\theta_{2,j,i} \in
\mathcal{S}_2,a_j\neq A_t
\end{cases}
\end{equation}

Q.E.D$\square$
